# Supplementary material for: Shape-aware Semi-supervised 3D Semantic Segmentation for Medical Images
Source: arXiv:2007.10732 source file (2020-07-21)
Supplement: Supplementary file 1 [file supp.tex]

% % figure 1: model
% \begin{figure}[t!]
%     \includegraphics[width=\textwidth]{img/GeoSSNet.png}
%     \caption{Illustration of the pipeline of our method. Input volumes are fed into a segmentation network, 
%     to predict 3D Signed Distance Maps (SDM) and segmentation maps. Then the generated SDM together with input 
%     volumes are taken by a discriminator, in purpose of classifying the volumes into labeled or unlabeled. 
%     } 
%     \label{fig:model}
% \end{figure}

% % figure 2: la_2d
% \begin{figure}[thb]
%     \includegraphics[width=\textwidth]{img/la_v1.png}
%     \caption{Qualitative segmentation comparison on left atrium segmentation test set. The first two columns 
%     presents original images and groundtruth segmentation respectively. The third and last columns show 
%     segmentation comparison of UA-MT and our GeoSSNet. Our GeoSSNet retains the global organ shape, generates 
%     complete and smooth masks. 
%     } 
%     \label{fig:la_vis2d}
% \end{figure}

% % figure 3: la_3d
% \begin{figure}[thb]
%     \includegraphics[width=\textwidth]{img/la_v2.png}
%     \caption{Qualitative segmentation comparison on left atrium test set. The training set is split into 8 
%     labled and 72 unlabeld data, we visualize three cases in corresponding columns. Three rows correspond 
%     to segmentation of groundtruth (GT), UA-MT and GeoSSNet. Our GeoSSNet generates complete segmentation 
%     with great shape awareness, surpass UA-MT by a large gap.
%     } 
%     \label{fig:la_vis3d}
% \end{figure}

% % figure 4: pan_2d
% \begin{figure}[thb]
%     \includegraphics[width=\textwidth]{img/pan_v1.png}
%     \caption{Qualitative segmentation comparison on pancreas test set. We train networks under the setting 
%     of 16 labeled and 46 unlabeled data, we present 3D visualization of three samples in correponding columns. 
%     For each column, three rows illustate segmentation of groundtruth (GT), V-Net and our model respectively. 
%     Our GeoSSNet produces segmentation with smooth surface and captures the global shape well.
%     } 
%     \label{fig:pan_vis3d}
% \end{figure}

% % table 1
% \begin{table}[htb]
%     \caption{Quantitative comparison of segmentation models on the Atrial Segmentation Challenge dataset. All models use V-Net as backbone. DAN denotes the deep adversarial network, and UA-MT denotes the uncertainty-aware mean-teacher framework. Our GeoSSNet outperforms state-of-the-art results by a large margin.}
%     \label{tab:la_16}
%     \begin{tabular}{c|c|c|c|c|c|c} \hline \hline
%     \multirow{2}{*}{Method} & \multicolumn{2}{c|}{\# \textbf{scans used}} & \multicolumn{4}{c}{\textbf{Metrics}}  \\ \cline{2-7}
%                             & Labeled        & Unlabeled        & Dice{[}\%{]} & Jaccard{[}\%{]} & ASD{[}voxel{]} & 95HD{[}voxel{]} \\ \hline
%     V-Net                   & 80             & 0                & 91.14        & 83.82           & 1.52           & 5.75            \\ \hline
%     V-Net                   & 16             & 0                & 86.03        & 76.06           & 3.51           & 14.26           \\ \hline
%     DAN                     & 16             & 64               & 87.52        & 78.29           & 2.42           & 9.01            \\ \hline
%     UA-MT                   & 16             & 64               & 88.88        & 80.21           & 2.26           & 7.32            \\ \hline
%     UA-MT(+NMS)	          & 16             & 64               & 89.11        & 80.62           & 2.21           & \textbf{7.30}            \\ \hline
%     GeoSSNet(ours)          & 16             & 64               & 89.27        & 80.82           & 3.13           & 8.83            \\ \hline
%     GeoSSNet(+NMS)          & 16             & 64               & \textbf{89.54}        & \textbf{81.24}           & \textbf{2.20}           & 8.24            \\ \hline  \hline
%     \end{tabular}
%     \end{table}

% % table 2
% \begin{table}[htb]
%     \caption{Quantitative analysis of our method when decreasing the labeled number by a half. Our method shows a more significant improvement, validating the importance of geometric awareness for semi-supervised semantic segmentation.}
%     \label{tab:la_08}
%     \begin{tabular}{c|c|c|c|c|c|c} \hline \hline
%         \multirow{2}{*}{Method} & \multicolumn{2}{c|}{\# \textbf{scans used}} & \multicolumn{4}{c}{\textbf{Metrics}}  \\ \cline{2-7}
%                             & Labeled        & Unlabeled        & Dice{[}\%{]} & Jaccard{[}\%{]} & ASD{[}voxel{]} & 95HD{[}voxel{]} \\ \hline
%     V-Net          & 8 & 0  & 79.99 & 68.12 & 5.48 & 21.11 \\ \hline
%     UAMT           & 8 & 72 & 84.25 & 73.48 & 3.36 & 13.84 \\ \hline
%     UAMT(+NMS)	 & 8 & 72 & 84.57 & 73.96 & 2.90 & 12.51 \\ \hline  
%     GeoSSNet(ours) & 8 & 72 & 86.81 & 76.92 & 3.94 & 12.54 \\ \hline
%     GeoSSNet(+NMS) & 8 & 72 & \textbf{87.32} & \textbf{77.72} & \textbf{2.55} & \textbf{9.62}  \\ \hline \hline
%     \end{tabular}
%     \end{table}



% % table 3
% \begin{table}[htb]
%     \caption{Ablation study of our proposed method on the Atrial Segmentation Challenge dataset. The setting of 8 labeld and 72 unlabeld samples is employed. With V-Net as the backbone, V-Net+SDM denotes adding the SDM head and enforcing SDM consistencies, and V-Net+SDM+SDM denotes employing a GAN to enforce geometric constraints.}
%     \label{tab:la_ablation}
%     \begin{tabular}{l|c|c|c|c|c|c} \hline \hline
%         \multirow{2}{*}{Method} & \multicolumn{2}{c|}{\# \textbf{scans used}} & \multicolumn{4}{c}{\textbf{Metrics}}  \\ \cline{2-7}
%                             & Labeled        & Unlabeled        & Dice{[}\%{]} & Jaccard{[}\%{]} & ASD{[}voxel{]} & 95HD{[}voxel{]} \\ \hline
%     V-Net           & 8 & 0  & 79.99 & 68.12 & 5.48 & 21.11 \\ \hline
%     V-Net +SDM      & 8 & 72 & 84.97 & 74.14 & 6.12 & 22.20 \\ \hline
%     V-Net +SDM +GAN & 8 & 72 & 86.81 & 76.92 & 3.94 & 12.54 \\ \hline \hline
%     \end{tabular}
%     \end{table}


% % table 4
% \begin{table}[htb]
%     \caption{Quantitative improvements of our model on NIH pancreas dataset.The first row presents upper bound of performances. Our model achieve high performance gains in different semi-supervised settings.}
%     \label{tab:pan_exp}
%     \begin{tabular}{c|c|c|c|c|c|c} \hline \hline
%         \multirow{2}{*}{Method} & \multicolumn{2}{c|}{\# \textbf{scans used}} & \multicolumn{4}{c}{\textbf{Metrics}}  \\ \cline{2-7}
%                             & Labeled        & Unlabeled        & Dice{[}\%{]} & Jaccard{[}\%{]} & ASD{[}voxel{]} & 95HD{[}voxel{]} \\ \hline
%     V-Net    & 62 & 0  & 79.61 & 66.80 & 10.04 & 3.23 \\ \hline
%     V-Net    & 32 & 0  & 74.70 & 60.32 & 11.53 & 3.60 \\ \hline
%     GeoSSNet & 32 & 30 & 77.81 & 64.06 & 9.90  & 2.96 \\ \hline
%     V-Net    & 16 & 0  & 69.17 & 53.74 & 15.73 & 5.35 \\ \hline
%     GeoSSNet & 16 & 46 & 74.52 & 60.09 & 11.08 & 3.41 \\  \hline \hline
%     \end{tabular}
%     \end{table}


% % figure: vis_la
% \begin{figure}[thb]
%     \centering
%     \begin{subfigure}[b]{\linewidth}
%         \includegraphics[width=\linewidth]{img/la_v2d}
%         \caption{}
%     \end{subfigure}
%     \begin{subfigure}[b]{\linewidth}
%         \includegraphics[width=\linewidth]{img/la_v3d}
%         \caption{}
%     \end{subfigure}


%     \caption{Qualitative segmentation comparison on left atrium segmentation test set. (a)(b) shows 2D and 3D comparison respectively, where GT denotes groundtruth segmetnation. Our GeoSSNet generates complete segmentation with good global shape, surpass UA-MT by a large margin.
%     } 
%     \label{fig:la_vis2d}
% \end{figure}





%%%%%%%%%%%%%%%%%%%%%%%%%%%%%%%%%%%%%% intro %%%%%%%%%%%%%%%%%%%%%%%%%%%
% 1. modify citations in above paragraph, append what you need.
% 2. select two or three important methods, and describe them. I just write the conclusive ideas.
% 3. here add referenced paper in Table 1
%adopt adversarial learning \cite{zhang2017deep,hung2018adversarial,nie2018asdnet,zheng2019semi} to force segmentation of unlabeled data look like segmentation of labeled data or groudtruth. \cite{zhang2017deep} introduced an evaluation network to force segmentation of unlabeled image look like segmentation of labeled image. \cite{hung2018adversarial} and \cite{nie2018asdnet} utilized adversarial learning to generate confidence map, and select the pixel of unlabeled image with high confidence to retrain the model. The other stream follows consistency regularization method \cite{laine2016temporal,tarvainen2017mean}, which force the models' prediction to be consistent under the random perturbation. \cite{laine2016temporal} encourage model's prediction to be consistency in temporal. \cite{tarvainen2017mean} encourage the student's prediction consistent with teacher's prediction under random noise and dropout. \cite{bortsova2019semi,li2018semi} encourage the student's prediction consistenct with teachers under different transformation. \cite{yu2019uncertainty} explore uncertainty in mean-teacher, and introduced an uncertainty map to guide student's learning. Although above make a success, they little take geometric constraint into consideration, which is vital important in medical image. 


%Traditional segmentation approaches adopt post processing for smooth and continuous shape.To incorporate geometric regularizations into neural networks, recently some approaches are proposed. Based on distance transform, Kervadec et al. \cite{kervadec2018boundary} reformulates a boundary loss term as a regional integral, and Karimi et al. \cite{D_HDloss_2020} designs a hausdorff loss, which provide complementary information to regional losses.Besides simply adding an extra boundary-aware loss, to capture the overall shape of the target organs, 
%Xue et al. \cite{xue2019shape} converts the segmentation task into predicting an signed distance map, which encodes richer structure information. In semi-supervised learning, Zheng et al. \cite{zheng2019semi} incorporates Deep Atlas Prior (DAP) in semi-supervised segmentation, so as to embed prior information such as shape and position into the model. 
%However, the assumption that organs have stable position priors is no longer valid when facing organs with complex or varied shape. 
